# Supplementary material for: Charge-parity switching effects and optimisation of transmon-qubit design parameters
Source: arXiv:2309.17168 source file (2024-03-29)
Supplement: Supplementary file 1 [file SupplementaryInformation.pdf]

# Supplementary Information:
# Charge-parity switching effects and optimisation of transmon-qubit design parameters

Miha Papič,[1,2,*] Jani Tuorila,[3] Adrian Auer,[1] Inés de Vega,[1,2] and Amin Hosseinkhani[1,†]

[1] *IQM, Georg-Brauchle-Ring 23-25, 80992 Munich, Germany*
[2] *Department of Physics and Arnold Sommerfeld Center for Theoretical Physics, Ludwig-Maximilians-Universität München, Theresienstr. 37, 80333 Munich, Germany*
[3] *IQM, Keilaranta 19, 02150 Espoo, Finland*

(Dated: March 27, 2024)

## NUMERICAL RESULTS BEYOND THE PERTURBATIVE REGIME

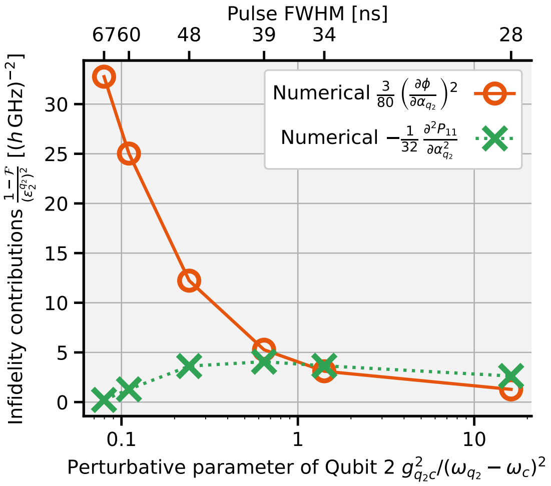


FIG. S1. The non-perturbative regime where the perturbative results derived in the previous section break down and leakage errors become the main error manifestation of the parity switch. The bottom $x$-axis shows the perturbative parameter, thus indicating the region where the perturbative results are no longer valid, while the upper $x$-axis shows the full-width-half-maximum of the flattop-Gaussian pulse of the individual points. The $y$-axis corresponds to the gate infidelity divided by the square of the charge dispersion of the second qubit. The parameters of the Hamiltonian for this simulation are given by Table 2 in the main text and are identical the ones from Fig. 2, with the exception that the conditional phases are no longer equal to $\pi$.

While we have established the effects of parity switches on the fidelity of a two-qubit gate in the main text, the derived results are valid in the perturbative regime. In order to see what happens when we move beyond the perturbative regime, we have simulated even faster gates, where the coupler must be tuned even closer to the qubit frequency. Since the perturbative results are valid up to second order in the parameter $g_{q_2c}^2/(\omega_{q_2}-\omega_c)^2$, we can see when the perturbative results are no longer valid by plotting this parameter on the $x$-axis of Fig. S1.

In the numerical simulations at shorter gate times, it can become difficult to find gate parameters with high fidelities, so the conditional phase requirement, $\phi_0=\pi$, was relaxed slightly, and the gates plotted in Fig. S1 are CPHASE gate rather than specifically CZ gates. What is evident from Fig. S1 is how the transition from the perturbative regime on the left to the non-perturbative regime changes the relative contributions of the parity-switch-induced leakage and phase errors. As the leakage errors, that were previously neglected in the perturbative regime (see Fig. 2b in the main text), become comparable to the conditional phase errors. All of the points in Fig. S1 were simulated with the same Hamiltonian parameters as in Fig. 2b, but with different pulse amplitudes and durations.

* miha.papic@meetiqm.com
† amin.hosseinkhani@meetiqm.com

The $y$-axis on this plot represents the contribution to the optimal process infidelity of the gate divided by the square of the charge dispersion. This is done so that the presented curves depend only on the gate parameters (including the parameters of the pulse) and not on the individual transmon $E_J$ and $E_C$. In order to obtain the infidelity contribution, the values on the $y$-axis must be multiplied by the square of the second qubits' charge dispersion, which is still the main source of the perturbation, due to the fact that the $f$-state is populated during the gate operation. Identically as in the perturbative regime, the larger charge dispersion of the second excited state means that the main effect of the parity switch is on the Rabi oscillation used to implement a gate. Therefore, we can *numerically* evaluate the quantities $\partial\phi/\partial\alpha_{q_2}$ and $\partial^2 P_{11}/\partial\alpha_{q_2}^2$, in order to probe the effect on the infidelity depending on the gate duration, rather than transmon parameters.

Both numerical derivatives were evaluated with standard finite difference formulas, and are expected to be representative, within an order of magnitude, for most implementations of the CPHASE gate.

## FIDELITY LIMITATIONS IN THE UNITARY SIMULATION

In this section we study the remaining gate infidelity in the noiseless unitary simulation, i.e. we are interested in the grey area of Fig. 2b.

There are different possible errors in the unitary simulation of the CZ gate. For example, it is possible that the CPHASE angle is not exactly equal to $\pi$. However, in the examples from Fig. 2b numerical data shows that $1-\mathcal{F} \propto (\pi-\phi)^2 \sim 10^{-8}$, and this error is too small to explain the $10^{-6}$ infidelity.

Leakage errors outside of the computational subspace, are another possible source of error. We observe that $1 - \mathrm{tr}\{\Pi\rho\} \sim 10^{-8}$, where $\Pi$ is the projector onto the computational subspace. The value of $10^{-8}$ is too small to explain the $\sim 10^{-6}$ infidelity.

This means that we are dealing with unwanted transitions within the computational subspace. A possible explanation is the residual iSWAP interaction between the $|01\rangle \leftrightarrow |10\rangle$ Rabi oscillation. Propagating the state $|\psi(t=0)\rangle = \frac{1}{2}(|00\rangle + |01\rangle + |10\rangle + |11\rangle)$ and extracting the populations of the computational states we observe that $|\langle 01|\psi(T)\rangle|^2 - 0.25 \sim 10^{-6}$ and $|\langle 10|\psi(T)\rangle|^2 - 0.25 \sim -10^{-6}$. Since the order of magnitude matches the magnitude of the infidelity, we can assume that an unwanted transition between the states 01 and 10 should explain the remaining infidelity. We then attempted to improve the fidelity by additionally applying the unitary $\exp(i\theta(XX+YY))$ to the final state $|\psi(T)\rangle$. However, this procedure did not improve the fidelity significantly, and the fitted iSWAP angle $\theta \sim 10^{-4}$ is too small to explain the $10^{-6}$ infidelity.

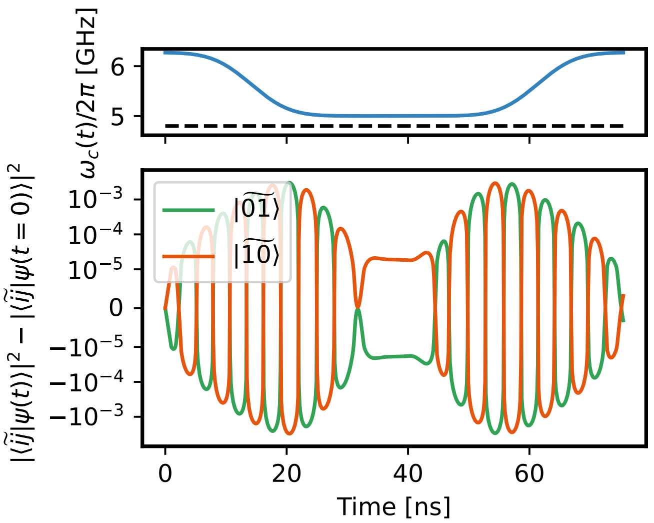


FIG. S2. *Upper panel*: The coupler frequency during a diabatic two-qubit gate. The black dashed line marks the frequency of Qubit 2 $\omega_{q_2}$. *Lower panel*: The population of the *instantaneous* Hamiltonian eigenstates corresponding to the single-excitation computational states during the operation of a two-qubit gate. The initial state was $|\psi(0)\rangle = (1,1,1,1)^T$. In order to highlight the errors we subtract the population at $t = 0$ and plot in the logarithmic scale. The gate parameters used in this plot correspond to the last point with highest $E_J/E_C$ on Fig. 2 in the main text.

The final source of error we consider are the unwanted diabatic transitions during the pulse ramping up and down.

To analyze this further, we monitor the populations of the *instantaneous* Hamiltonian eigenstates $|\langle\psi(t)|\widetilde{01}\rangle|^2$ and $|\langle\psi(t)|\widetilde{10}\rangle|^2$. These results are plotted on Fig. S2. In the completely adiabatic case, both quantities on the lower panel of Fig. S2 are equal to zero. We observe coherent population oscillation between the instantaneous computational basis states $|\widetilde{01}\rangle$ and $|\widetilde{10}\rangle$. The population swapping only occurs during the pulse ramping up and down, and almost completely stops in the plateau phase when the Hamiltonian is constant in time. We observe that after the ramping up phase of the pulse, in the center of Fig. S2, a small population exchange between the states due to undesired diabatic transitions has occurred.

## INFIDELITY DUE TO $1/f$-TYPE CHARGE NOISE

Increasing the charge dispersion of the transmon will also result in an increased sensitivity of the circuit to $1/f$-type charge noise[1]. This effect manifests itself as a contribution to the pure dephasing rate of the transmon. More specifically, we can write [1],

$$\Gamma_{\phi,m} = \frac{A_Q}{\hbar}\left|\frac{\partial E_m}{\partial n_g}\right| \simeq \frac{A_Q\pi|\epsilon_m \sin(2\pi n_g)|}{\hbar}, \tag{S1}$$

where $A_Q$ is the amplitude of the charge noise spectrum, assumed to have the form $S_Q(\omega) = 2\pi A_Q^2/|\omega|$ and $\Gamma_{\phi,m}$ is used to denote the pure dephasing rate associated with the $m$-th excited level of the transmon. While the decay rate also depends on the exact value of the offset charge $n_g$, we will at this point assume that $\sin(2\pi n_g) = 1$, as the worst-case scenario. Since the uncontrolled charged environment of the transmon will result in stochastic fluctuations of $n_g$ over longer timescales, as was demonstrated in Refs. [2, 3], we cannot assume that the decoherence rate in Eq. S1 can be set to zero. However even if this were hypothetically possible, the value of $n_g$ at which the decay rates from Eq. S1 are $\Gamma_{\phi,m} = 0$ is determined by the condition $\sin(2\pi n_g) = 0$. On the other hand, the value of $n_g$ at which the charge dispersion of the transmon from Eq. 3 is zero is determined by the condition $\cos(2\pi n_g) = 0$. This means that at the value of $n_g$ where the effects of the charge-parity switching error is minimized corresponds to the largest infidelity contribution of the charge noise and vice versa. In order to estimate the infidelity, we will neglect the time-correlated nature of the $1/f$ noise and assume the dynamics of a single transmon are Markovian, and thus described by the following set of jump operators

$$\hat{L}_m = \sqrt{\Gamma_{\phi,m}}\,\mathrm{diag}(0,\dots,0,\underbrace{1}_{m},0,\dots,0). \tag{S2}$$

We mention here that neglecting the time correlations of the noise and approximating it as a Markovian process means that the derived results can only be used to qualitatively asses the impact on the infidelity as an order of magnitude approximation. The pure dephasing decay, as measured by a Ramsey experiment, produced by a time-correlated $1/f$-type noise will result in a Gaussian type decay, rather than the exponential predicted by the Lindblad equation[4]. This means that the Markovian approximation will overestimate the infidelity contribution at small times, i.e. when $\Gamma_\phi t \ll 1$ and underestimate the decay at longer timescales when $\Gamma_\phi t \gg 1$. Moreover, the process infidelity of a gate in the presence of time correlations is not a well-defined quantity, as the gate performance depends on the history (i.e. any potential previously applied gates). However, by analyzing the process infidelity of a single gate, i.e. assuming perfect state preparation, since the gate duration $t_g$ is typically much shorter compared to the decoherence rate $\Gamma_\phi$, we are typically in the regime where $\Gamma_\phi t_g \ll 1$ and thus the Markovian approximation provides an upper bound.

In order to account for the contribution of the charge noise to the pure dephasing decay both in the computational subspcae and the employed higher states, we employ the formalism developed in Ref. [5]. We will assume the perturbative approximation holds and employ the effective Hamiltonian from Eq. 37 with the identical assumption of a square pulse with duration $t_g$. By further assuming the $|11\rangle$ and $|02\rangle$ states are resonant, i.e. $\tilde{\omega}_{q_1} + \tilde{\omega}_{q_2} = 2\tilde{\omega}_{q_2} + \tilde{\alpha}_{q_2}$, which is beneficial, since it results in shorter gate durations. The full unitary obtained by exponentiating the Hamiltonian from Eq. 37 is given by

$$\begin{aligned}\hat{U}_{\mathrm{eff}}(t) &= |00\rangle\langle 00| + |10\rangle\langle 10| + |01\rangle\langle 01| \\ &\quad + \cos(\tilde{g}_{11,02}t)\left(|11\rangle\langle 11| + |02\rangle\langle 02|\right) - i\sin(\tilde{g}_{11,02}t)\left(|11\rangle\langle 02| + |02\rangle\langle 11|\right)\end{aligned} \tag{S3}$$

where we have removed the single-qubit phases, however we have not truncated the Hilbert space to the computational states.

Following Ref. [5], the infidelity of the gate, due to the charge noise acting on the computational transmons $(q_{1,2})$ and the first two excited states is given by

$$1 - \mathcal{F}_{1/f} = \sum_{(i,m)\in\{(q_1,1),(q_2,1),(q_2,2)\}} \int_0^{t_g} \mathrm{d}\tau\, \delta F(\tau, \hat{L}_m^i) + \mathcal{O}\left(\left[\Gamma_{\phi,m}^i t_g\right]^2\right). \tag{S4}$$

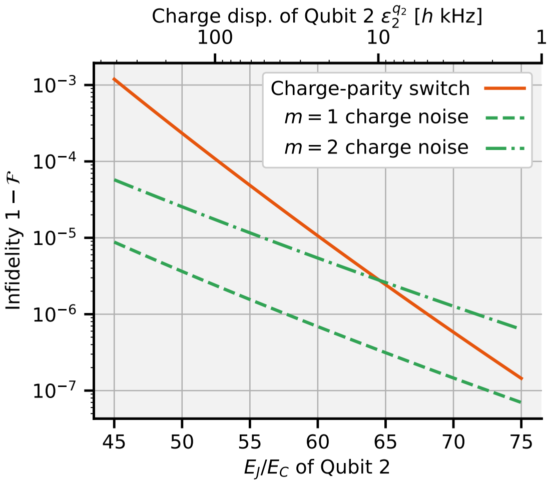


FIG. S3. Comparison of the gate infidelity due to a charge-parity switch, as defined in Eq. 16 (orange solid line) and the infidelity due to $1/f$-type charge noise (green), where we have separated the contribution from the computational space dephasing (dashed line), i.e. terms proportional to $\Gamma_{\phi,1}^{q_1,2}$, and the $|02\rangle$ dephasing (dash-dotted line), i.e. terms proportional to $\Gamma_{\phi,2}^{q_2}$. The charging energy was fixed at $E_C = 0.2\,h\,\text{GHz}$, while the Josephson energy $E_J$ was varied along the $x$-axis. The gate time was chosen to be $t_g = 60\,\text{ns}$, while the charge noise amplitude was set to $A_Q = 10^{-4}$, as in Ref. [1].

where $\hat{L}_1^{q_1} = \sqrt{\Gamma_{\phi,1}^{q_1}}\,(|10\rangle\langle 10| + |11\rangle\langle 11|)$, $\hat{L}_1^{q_2} = \sqrt{\Gamma_{\phi,1}^{q_2}}\,(|01\rangle\langle 01| + |11\rangle\langle 11|)$ and $\hat{L}_2^{q_2} = \sqrt{\Gamma_{\phi,2}^{q_2}}|02\rangle\langle 02|$, and the quantity $\delta F(\tau, \hat{L}_m^i)$ is calculated by

$$\delta F(t, \hat{L}_m^i) = \frac{1}{20}\mathrm{tr}_{\mathrm{cmp}}\left[\hat{L}_m^i(t)\right]\mathrm{tr}_{\mathrm{cmp}}\left[\hat{L}_m^i(t)^\dagger\right] - \frac{1}{5}\left[\hat{L}_m^i(t)^\dagger \hat{L}_m^i(t)\right], \tag{S5}$$

where $\hat{L}_m^i(t)$ is the time evolved operator with respect to the unitary in Eq. S3, i.e. $\hat{L}_m^i(t) = \hat{U}_{\mathrm{eff}}(t)^\dagger\,\hat{L}_m^i\,\hat{U}_{\mathrm{eff}}(t)$. The notation $\mathrm{tr}_{\mathrm{cmp}}\,[\cdot]$ denotes the trace over the computational subspace, i.e. the states $\{|00\rangle, |01\rangle, |10\rangle, |11\rangle\}$.

Evaluating the expression in Eq. S5 with the explicit forms for $\hat{U}_{\mathrm{eff}}(t)$ from Eq. S3 and the expressions for $\hat{L}_m^i$, we arrive at

$$1 - \mathcal{F}_{1/f} = \frac{13}{160}\Gamma_{\phi,2}^{q_2} t_g + \frac{29}{160}\Gamma_{\phi,1}^{q_2} t_g + \frac{29}{160}\Gamma_{\phi,1}^{q_1} t_g, \tag{S6}$$

which we further simplify by assuming both qubits have similar charge dispersions $\epsilon_1^{q_1} = \epsilon_1^{q_1} = \epsilon_1$ and the same charge noise amplitude $A_Q^{q_1} = A_Q^{q_2} = A_Q$,

$$1 - \mathcal{F}_{1/f} \approx \frac{A_Q \pi}{160}\left(13\frac{|\epsilon_2| t_g}{\hbar} + 58\frac{|\epsilon_1| t_g}{\hbar}\right). \tag{S7}$$

In order to take into account the stochastic nature of the fluctuations in $n_g$ we can assume that the value of $n_g$ is uniformly distributed in the interval $[0, 1]$, thus the infidelity from Eq. S7 averaged over $n_g$ will be additionally reduced by a factor of $\int_0^1 \mathrm{d}n_g |\sin(2\pi n_g)| = 2/\pi$. Furthermore, Eq. S7 was used to compare the effects of the charge noise with the parity-switch induced infidelity in Fig. S3. We can see that the charge noise infidelity is dominated by the higher-excited state contribution $\Gamma_{\phi,1}^{q_2}$, which is again due to $|\epsilon_2/\epsilon_1| \sim 50$. It is also evident that the charge-parity error is dominant at lower $E_J/E_C$, thus demonstrating that the charge parity mechanism will limit the $E_J/E_C$ ratio of a transmon more than the susceptibility to charge noise, as other error sources (such as $T_1$) will typically dominate the infidelity at larger $E_J/E_C$, due to the exponential suppression of both errors considered in this section. As an example, in order to achieve an infidelity on the order of $1 - \mathcal{F} \sim 10^{-6}$, a $T_1$ time on the order of 10 ms is required, as per the results in Table 1.

We also note that in our analysis the coupler charge noise was assumed to be negligible, due to the typically much larger $E_{J_c}/E_{C_c} \sim 100$[6, 7]. If, however, this is not the case, such as for the parameters in Ref. [8], the hybridization of the computational basis with the transmon modes must be taken into account, as was described in Ref. [9].

## ADIABATIC INTERACTION - FURTHER NUMERICAL RESULTS

Here we present further numerical data analyzing the contributions to the adiabatic ZZ coupling rate $\zeta_{\rm ZZ}$ at larger qubit detunings. The adiabatic coupling strength is plotted in the upper left panel of Fig. S4, clearly showing the three detuning regimes with two, one and zero coupler idling frequencies (i.e. values of $\omega_c$ where $\zeta^0_{\rm ZZ} = 0$). The remaining panels in Fig. S4 display the three largest contributions to the charge-parity switch susceptibility of the coupling strength, as displayed in Fig. 3a of the main text. Unlike the derivatives $\partial\zeta_{\rm ZZ}/\partial\omega_{q_{1,2}}$, the largest contribution resulting from the hybridization with the second-excited state of the high-frequency computational transmon $\partial\zeta_{\rm ZZ}/\partial\alpha_{q_2}$ has no zero points.

Since the considered couplings are symmetric (i.e. $\beta_{q_1c} = \beta_{q_2c}$) and the anharmonicities of the computational transmons are similar (i.e. $\alpha_{q_1} \approx \alpha_{q_2}$), the lower panels displaying $\partial\zeta_{\rm ZZ}/\partial\omega_{q_{1,2}}$ are almost symmetric about the $\omega_{q_1} - \omega_{q_2} = 0$ line, and a similar symmetry is observed in the derivative $\partial\zeta_{\rm ZZ}/\partial\alpha_{q_1}$ (not plotted), which is irrelevant at the detuning considered in Fig. 3a. This symmetry can also be seen by switching the indices of the computational transmons $q_1 \leftrightarrow q_2$, since positive detunings imply that Qubit 1 ($q_1$) is the high-frequency computational transmon. This symmetry also means that close to the zero detuning line, both $\partial\zeta_{\rm ZZ}/\partial\alpha_{q_1}$ and $\partial\zeta_{\rm ZZ}/\partial\alpha_{q_2}$ will contribute almost equally to the parity-switching-induced fluctuations of the ZZ coupling strength and adiabatic gate infidelity. In this case the formula for the fidelity of the adiabatic CPHASE gate is generalized to

$$\mathcal{F} \approx 1 - \frac{3}{80}\frac{t_g^2}{\hbar^2}\left[\left(\frac{\partial\zeta_{\rm ZZ}}{\partial\alpha_{q_2}}\epsilon_2^{q_2}\cos(2\pi n_g^{q_2})\right)^2 + \left(\frac{\partial\zeta_{\rm ZZ}}{\partial\alpha_{q_1}}\epsilon_2^{q_1}\cos(2\pi n_g^{q_1})\right)^2\right], \tag{S8}$$

where we have ignored the contributions from $\partial\zeta_{\rm ZZ}/\partial\omega_{q_{1,2}}$, which are close to zero in the zero detuning regime, as seen from the bottom panels in Fig. S4, as well as any higher order contributions. In the derivation of Eq. S8, we have assumed the same separation of timescales as in the derivations for all the previous fidelity formulas, however the noisy dynamics in this case are described by four instead of two Kraus operators, corresponding to the four relevant parity states of the system.

Even though the infidelity has two contributions in the zero detuning regime, the values of $\partial\zeta_{\rm ZZ}/\partial\omega_{q_{1,2}}$ are much smaller compared to the regime where the detuning is close to the relevant anharmonicity, thus implying that fixing $\omega_{q_1} = \omega_{q_2}$ will reduce the susceptibility of an adiabatic gate to charge-parity switches. Nonetheless, the zero detuning regime is also associated with weaker values of the coupling strength $\zeta^0_{\rm ZZ}$[8], thus implying that this regime is unfavorable due to longer gate durations $t_g$ and therefore more decoherence. The right balance between the charge-parity switching error and the decoherence in an adiabatic gate will therefore depend on the exact details such as the coherence rates, and $E_J/E_C$ ratios of the transmons.

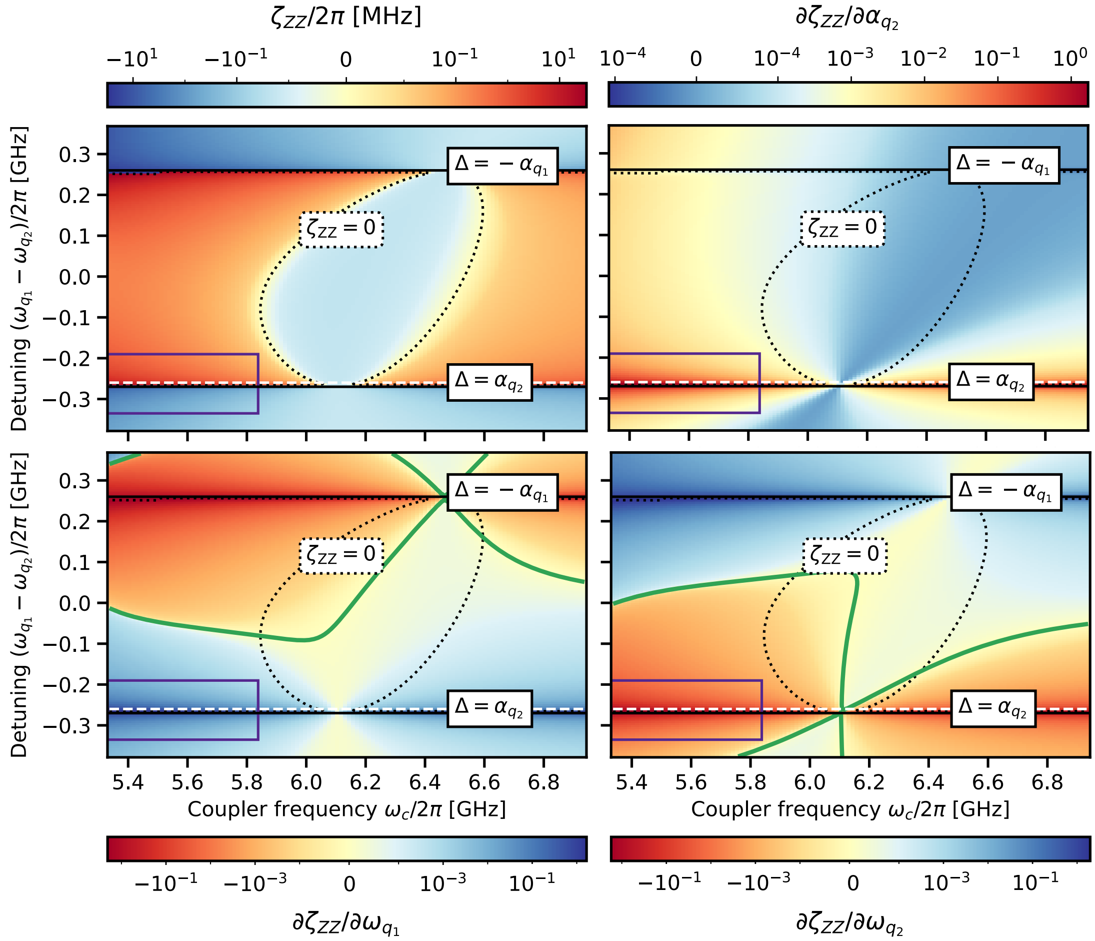


FIG. S4. *Upper left*: The ZZ coupling strength $\zeta_{\mathrm{ZZ}}$, defined in Eq. 20 in the main text depending on the frequency of the coupler ($x$-axis) and the qubit-qubit detuning $\Delta = \omega_{q_1} - \omega_{q_2}$ ($y$-axis). The dotted contour represents the switch between $\zeta_{\mathrm{ZZ}} > 0$ and $\zeta_{\mathrm{ZZ}} < 0$, with the elliptical region in the center corresponding to $\zeta_{\mathrm{ZZ}} = 0$. The white dashed line marks the detuning used in Fig. 3a in the main text. The horizontal black lines correspond to the special cases where $\Delta = \omega_{q_1} - \omega_{q_2} = -\alpha_{q_1}$ or $\alpha_{q_2}$, as indicated on the plot. The purple rectangle displays part of the region plotted in Fig. 3c in the main text. *Upper right*: Numerically computed value of the derivative $\partial\zeta_{\mathrm{ZZ}}/\partial\alpha_{q_2}$. *Lower left*: Numerically computed value of the derivative $\partial\zeta_{\mathrm{ZZ}}/\partial\omega_{q_1}$. *Lower right*: Numerically computed value of the derivative $\partial\zeta_{\mathrm{ZZ}}/\partial\omega_{q_2}$. The green line on both lower plots corresponds to $\partial\zeta_{\mathrm{ZZ}}/\partial\omega_{q_{1,2}} = 0$. The parameters used in this figure correspond to the same set as in Fig. 3a and c in the main text. Each panel contains $120 \times 160$ pixels.


[1] J. Koch, T. M. Yu, J. Gambetta, A. A. Houck, D. I. Schuster, J. Majer, A. Blais, M. H. Devoret, S. M. Girvin, and R. J. Schoelkopf, Charge-insensitive qubit design derived from the cooper pair box, Phys. Rev. A **76**, 042319 (2007).

[2] B. G. Christensen, C. D. Wilen, A. Opremcak, J. Nelson, F. Schlenker, C. H. Zimonick, L. Faoro, L. B. Ioffe, Y. J. Rosen, J. L. DuBois, B. L. T. Plourde, and R. McDermott, Anomalous charge noise in superconducting qubits, Phys. Rev. B **100**, 140503 (2019).

[3] C. D. Wilen, S. Abdullah, N. A. Kurinsky, C. Stanford, L. Cardani, G. D'Imperio, C. Tomei, L. Faoro, L. B. Ioffe, C. H. Liu, A. Opremcak, B. G. Christensen, J. L. DuBois, and R. McDermott, Correlated charge noise and relaxation errors in superconducting qubits, Nature **594**, 369 (2021).

[4] E. Paladino, Y. M. Galperin, G. Falci, and B. L. Altshuler, $1/f$ noise: Implications for solid-state quantum information, Rev. Mod. Phys. **86**, 361 (2014).

[5] T. Abad, A. F. Kockum, and G. Johansson, Impact of decoherence on the fidelity of quantum gates leaving the computational subspace (2023), arXiv:2302.13885 [quant-ph].

[6] Y. Sung, L. Ding, J. Braumüller, A. Vepsäläinen, B. Kannan, M. Kjaergaard, A. Greene, G. O. Samach, C. McNally, D. Kim, A. Melville, B. M. Niedzielski, M. E. Schwartz, J. L. Yoder, T. P. Orlando, S. Gustavsson, and W. D. Oliver, Realization of high-fidelity cz and $zz$-free iswap gates with a tunable coupler, Phys. Rev. X **11**, 021058 (2021).

[7] J. Chu and F. Yan, Coupler-assisted controlled-phase gate with enhanced adiabaticity, Phys. Rev. Appl. **16**, 054020 (2021).
[8] F. Marxer, A. Vepsäläinen, S. W. Jolin, J. Tuorila, A. Landra, C. Ockeloen-Korppi, W. Liu, O. Ahonen, A. Auer, L. Belzane, V. Bergholm, C. F. Chan, K. W. Chan, T. Hiltunen, J. Hotari, E. Hyyppä, J. Ikonen, D. Janzso, M. Koistinen, J. Kotilahti, T. Li, J. Luus, M. Papic, M. Partanen, J. Räbinä, J. Rosti, M. Savytskyi, M. Seppälä, V. Sevriuk, E. Takala, B. Tarasinski, M. J. Thapa, F. Tosto, N. Vorobeva, L. Yu, K. Y. Tan, J. Hassel, M. Möttönen, and J. Heinsoo, Long-distance transmon coupler with cz-gate fidelity above 99.8%, PRX Quantum **4**, 010314 (2023).
[9] M. Papič, A. Auer, and I. de Vega, Fast estimation of physical error contributions of quantum gates (2023), arXiv:2305.08916 [quant-ph].
